# Supplementary material for: Time-Sliced Perturbation Theory II: Baryon Acoustic Oscillations and Infrared Resummation
Source: arXiv:1605.02149 source file (2016-07-19)
Supplement: Supplementary file 1 [file supp-mis.tex]

%D \module
%D   [       file=supp-mis,
%D        version=1997.01.04,
%D          title=\CONTEXT\ Support Macros,
%D       subtitle=Missing (For Generic Use),
%D         author=Hans Hagen,
%D           date=\currentdate,
%D      copyright={PRAGMA / Hans Hagen \& Ton Otten}]
%C
%C This module is part of the \CONTEXT\ macro||package and is
%C therefore copyrighted by \PRAGMA. See mreadme.pdf for 
%C details. 

%D Some support modules are more or less independant. This
%D module, which is not part of plain \CONTEXT, provides the
%D missing macros and declarations of registers.

\ifx \undefined \writestatus \else \expandafter \endinput \fi

\ifx \undefined \pdfoutput \chardef\pdfoutput=0 \fi 

%D Because \LATEX\ has no safe package loading mechanism, we
%D need to take care of possible interference. 

\def\StartLatexHack% 
  {\edef\StopLatexHack
     {\catcode`\noexpand/=\the\catcode`/ 
      \catcode`\noexpand:=\the\catcode`:
      \catcode`\noexpand;=\the\catcode`;
      \catcode`\noexpand"=\the\catcode`"
      \catcode`\noexpand<=\the\catcode`< 
      \catcode`\noexpand>=\the\catcode`>}%
  \catcode`/=12 \catcode`:=12 \catcode`;=12 
  \catcode`"=12 \catcode`<=12 \catcode`>=12 }

%D This hack is needed especially for \LATEX\ users who use
%D the Babel package. The Germans have active \type {"}'s, the
%D Poles have \type {/}, while the French have \type {:} and
%D \type {;} defines as command (thanks to Daniel Flipo for
%D pointing that out and testing). Potentially active \type
%D {?}'s and \type {!}'s are less dangerous since they are
%D handled by the \type {\protect} and \type {\unprotect}
%D macros. 

\StartLatexHack

%D \macros
%D   {ifnocontextobject}
%D
%D First we take care of redundant defining. The next set of
%D macros are a bit complicated by the fact that Plain
%D \TEX\ defines the \type{\new}||macros as being outer.
%D Furthermore nested \type{\if}'s can get us into
%D trouble.

\def\definecontextobject%
  {\iftrue}

\def\gobblecontextobject%
  {\setbox0=\hbox
     \bgroup
     \long\def\gobblecontextobject##1\fi{\egroup}%
     \expandafter\gobblecontextobject\string}

\long\def\ifnocontextobject#1\do%
  {\ifx#1\undefined
     \expandafter\definecontextobject
   \else
     %\writestatus{system}{beware of conflicting \string#1}%
     \expandafter\gobblecontextobject
   \fi}

%D \macros 
%D   {beginETEX,beginTEX}
%D
%D Outside \CONTEXT\ we will not be \ETEX||aware.

\long\def\beginETEX #1\endETEX {}
\long\def\beginOMEGA#1\endOMEGA{}

\let\beginTEX\relax \let\endTEX\relax

%D \macros
%D   {writestatus}
%D
%D We start each module with a message. Normally the output is
%D formatted, but here we keep things simple.

\ifnocontextobject \writestatus \do

  \def\writestatus#1#2%
    {\immediate\write16{#1 : #2}}

\fi

%D Lets see if it works.

\writestatus{loading}{Context Support Macros / Missing}

%D \macros
%D   {protect,unprotect}
%D
%D Next we present a poor mans alternative for \type{\protect}
%D and \type{\unprotect}, two commands that enable us to use
%D the characters \type{@}, \type{!} and \type{?} in macro
%D names.

\ifnocontextobject \protect \do

  \let\protect\relax

\fi

\newcount\protectiondepth

\ifnocontextobject \unprotect \do

  \def\unprotect%
    {\advance\protectiondepth 1
     \ifnum\protectiondepth=1
       \let\normalprotect=\protect
       \def\protect%
         {\ifnum\protectiondepth>0
            \advance\protectiondepth -1
            \ifnum\protectiondepth=0
              \doprotect
              \let\protect=\normalprotect
            \fi
          \fi}
       \edef\doprotect%
         {\catcode`\noexpand @=\the\catcode`@\relax
          \catcode`\noexpand !=\the\catcode`!\relax
          \catcode`\noexpand ?=\the\catcode`?\relax}
       \catcode`@=11
       \catcode`!=11
       \catcode`?=11
     \fi}

\fi

%D We start using this one it at once.

\unprotect

%D \macros
%D   {scratch...,if...,next...}
%D
%D We need some scratch registers. Users are free to use them,
%D but can never be sure of their value once another macro is
%D called. We only allocate things when they are yet
%D undefined. This way we can't mess up other macro packages,
%D but of course previous definitions can mess up our modules.

\ifnocontextobject \scratchcounter \do \newcount  \scratchcounter \fi
\ifnocontextobject \scratchtoks    \do \newtoks   \scratchtoks    \fi
\ifnocontextobject \scratchdimen   \do \newdimen  \scratchdimen   \fi
\ifnocontextobject \scratchskip    \do \newskip   \scratchskip    \fi
\ifnocontextobject \scratchmuskip  \do \newmuskip \scratchmuskip  \fi
\ifnocontextobject \scratchbox     \do \newbox    \scratchbox     \fi
\ifnocontextobject \scratchread    \do \newread   \scratchread    \fi
\ifnocontextobject \scratchwrite   \do \newwrite  \scratchwrite   \fi

\ifnocontextobject \zeropoint      \do \newdimen  \zeropoint      \fi
\ifnocontextobject \zerocount      \do \chardef   \zerocount=0    \fi
\ifnocontextobject \plusone        \do \chardef   \plusone  =1    \fi
\ifnocontextobject \minusone       \do \newcount  \minusone       \fi

\ifnocontextobject \thousandpoint  \do \newdimen  \thousandpoint  \fi

\thousandpoint=1000pt 
\minusone     = -1 

\ifnocontextobject \emptytoks      \do \newtoks   \emptytoks      \fi

\ifnocontextobject \nextbox   \do \newbox   \nextbox   \fi
\ifnocontextobject \nextdepth \do \newdimen \nextdepth \fi

\ifnocontextobject \CONTEXTtrue            \do \newif\ifCONTEXT            \fi
\ifnocontextobject \donetrue               \do \newif\ifdone               \fi
\ifnocontextobject \eightbitcharacterstrue \do \newif\ifeightbitcharacters \fi
\ifnocontextobject \MPdrawingdonetrue      \do \newif\ifMPdrawingdone      \fi

\ifnocontextobject \ifzeropt               \do \let\ifzeropt\ifcase        \fi

%D \macros
%D   {@@...}
%D
%D We use symbolic name for \CATCODES. They can only be used
%D when we are in unprotected state.

\ifnocontextobject \@@escape     \do \chardef\@@escape     =  0 \fi
\ifnocontextobject \@@begingroup \do \chardef\@@begingroup =  1 \fi
\ifnocontextobject \@@endgroup   \do \chardef\@@endgroup   =  2 \fi
\ifnocontextobject \@@endofline  \do \chardef\@@endofline  =  5 \fi
\ifnocontextobject \@@ignore     \do \chardef\@@ignore     =  9 \fi
\ifnocontextobject \@@space      \do \chardef\@@space      = 10 \fi
\ifnocontextobject \@@letter     \do \chardef\@@letter     = 11 \fi
\ifnocontextobject \@@other      \do \chardef\@@other      = 12 \fi
\ifnocontextobject \@@active     \do \chardef\@@active     = 13 \fi
\ifnocontextobject \@@comment    \do \chardef\@@comment    = 14 \fi

\def\s!sp{sp}
\def\s!pt{pt}
\def\s!bp{bp}

%D \macros 
%D   {@EA,expanded,expandoneargafter,expandtwoargsafter}
%D
%D Also needed: 

\let\@EA=\expandafter \let\@@expanded\empty

\def\expanded#1%
  {\long\xdef\@@expanded{\noexpand#1}\@@expanded}

\def\expandoneargafter#1#2%
  {\@EA#1\@EA{#2}}

\def\expandtwoargsafter#1#2#3%
  {\@EA\@EA\@EA#1\@EA\@EA\@EA{\@EA#2\@EA}\@EA{#3}}

\def\@EAEAEA{\@EA\@EA\@EA}

%D \macros
%D   {everyline,EveryLine,EveryPar}
%D
%D In \CONTEXT\ we use \type{\everypar} for special purposes
%D and provide \type{\EveryPar} as an alternative. The same
%D goes for \type{\everyline} and \type{\EveryLine}.

\ifnocontextobject \everyline \do \newtoks\everyline        \fi
\ifnocontextobject \EveryPar  \do \let\EveryPar =\everypar  \fi
\ifnocontextobject \EveryLine \do \let\EveryLine=\everyline \fi

%D \macros
%D   {globallet}

\def\globallet{\global\let}

%D \macros
%D   {!!...}
%D
%D We reserve ourselves some scratch strings (i.e. macros)
%D and some more counters.

\ifnocontextobject \!!stringa \do \def\!!stringa {} \fi
\ifnocontextobject \!!stringb \do \def\!!stringb {} \fi
\ifnocontextobject \!!stringc \do \def\!!stringc {} \fi
\ifnocontextobject \!!stringd \do \def\!!stringd {} \fi

\ifnocontextobject \!!counta \do \newcount\!!counta {} \fi
\ifnocontextobject \!!countb \do \newcount\!!countb {} \fi

%D \macros
%D   {!!...}
%D
%D The next set of definitions speed up processing a bit.
%D Furthermore it saves memory.

\ifnocontextobject \!!zeropoint   \do \def\!!zeropoint   {0pt}    \fi
\ifnocontextobject \!!zerocount   \do \def\!!zerocount   {0}      \fi
\ifnocontextobject \!!tenthousand \do \def\!!tenthousand {10000}  \fi

\ifnocontextobject \!!width       \do \def\!!width       {width}  \fi
\ifnocontextobject \!!height      \do \def\!!height      {height} \fi
\ifnocontextobject \!!depth       \do \def\!!depth       {depth}  \fi

\ifnocontextobject \!!plus        \do \def\!!plus        {plus}   \fi
\ifnocontextobject \!!minus       \do \def\!!minus       {minus}  \fi
\ifnocontextobject \!!to          \do \def\!!to          {to}     \fi

%D \macros
%D   {smashbox}
%D
%D The system modules offer a range of smashing macros, of
%D which we only copied \type{\smashbox}.

\ifnocontextobject \smashbox \do

  \def\smashbox#1%
    {\wd#1=\!!zeropoint
     \ht#1=\!!zeropoint
     \dp#1=\!!zeropoint}

\fi

%D \macros
%D   {dowithnextbox}
%D
%D Also without further comment, we introduce a macro that
%D gets the next box and does something usefull with it.
%D Because the \type{\afterassignment} is executed inside the
%D box, we have to use a \type{\aftergroup} too.

\ifnocontextobject \dowithnextbox \do

  \def\dowithnextbox#1%
    {\def\dodowithnextbox{#1}%
     \afterassignment\dododowithnextbox
     \setbox\nextbox}

  \def\dododowithnextbox%
    {\aftergroup\dodowithnextbox}

\fi

%D \macros
%D   {setvalue,setevalue,setxvalue,,setgvalue,
%D    getvalue,
%D    letvalue,letgvalue}
%D
%D The next two macros expand their argument to
%D \type{\argument}. The first one is used to define macro's
%D the second one executes them.

\ifnocontextobject \setvalue \do

  \def\setvalue #1{\expandafter\def\csname#1\endcsname}
  \def\setevalue#1{\expandafter\edef\csname#1\endcsname}
  \def\setgvalue#1{\expandafter\gdef\csname#1\endcsname}
  \def\setxvalue#1{\expandafter\xdef\csname#1\endcsname}
  \def\getvalue #1{\csname#1\endcsname}
  \def\letvalue #1{\expandafter\let\csname#1\endcsname}
  \def\letgvalue#1{\global\expandafter\let\csname#1\endcsname}
\fi

%D \macros
%D   {unexpanded}
%D
%D The next command can be used as prefixed for commands that
%D need protection during tests and writing to files. This
%D is a very \CONTEXT\ specific one.

\ifnocontextobject \unexpanded \do

  \let\unexpanded\relax

\fi

%D \macros
%D   {convertargument}
%D
%D The original one offers a bit more, like global assignment, the
%D the next implementation is however a bit more byte saving.

\ifnocontextobject \convertargument \do

  \def\doconvertargument#1>{}

  \long\def\convertargument#1\to#2%
    {\long\def\convertedargument{#1}%
     \edef#2{\expandafter\doconvertargument\meaning\convertedargument}}

\fi

%D \macros
%D   {forgetall}
%D
%D Sometimes we have to disable interference of whatever kind
%D of skips and mechanisms. The next macro resets some.

\ifnocontextobject \forgetall \do

  \def\forgetall%
    {\parskip\!!zeropoint
     \leftskip\!!zeropoint
     \parindent\!!zeropoint
     \everypar{}}

\fi

%D \macros
%D   {withoutpt,
%D    ScaledPointsToBigPoints,ScaledPointsToWholeBigPoints}
%D
%D \TEX\ lacks some real datastructure. We can however use
%D \DIMENSIONS. This kind of trickery is needed when we want
%D \TEX\ to communicate with the outside world (by means of
%D \type{\specials}).

\ifnocontextobject \withoutpt \do

  {\catcode`\.=\@@other
   \catcode`\p=\@@other
   \catcode`\t=\@@other
   \gdef\WITHOUTPT#1pt{#1}}

  \def\withoutpt#1%
    {\expandafter\WITHOUTPT#1}

  \def\ScaledPointsToBigPoints#1#2%
    {\scratchdimen=#1sp\relax
     \scratchdimen=.996264\scratchdimen
     \edef#2{\withoutpt{\the\scratchdimen}}}

  \def\ScaledPointsToWholeBigPoints#1#2%  
    {\scratchdimen=#1sp
     \scratchdimen=.996264\scratchdimen    
     \scratchcounter=\scratchdimen
     \advance\scratchcounter by 32768
     \divide\scratchcounter by 65536
     \edef#2{\the\scratchcounter}}

\fi

%D \macros
%D   {doprocessfile}
%D
%D This macro takes three arguments: the file number, the
%D filename and a macro that handles the content of a read
%D line.

\newif\iffileprocessed

\ifnocontextobject \doprocessfile \do

  \def\doprocessfile#1#2#3%
    {\openin#1=#2\relax
     \ifeof#1%
       \fileprocessedfalse
       \closein#1\relax
     \else
       \fileprocessedtrue
       \gdef\dofinishfile% 
         {\closein#1\relax
          \global\let\doprocessline\relax}%
       \gdef\doprocessline%
         {\ifeof#1%
            \dofinishfile
          \else
            \global\read#1 to \fileline
            #3\relax
            \expandafter\doprocessline
          \fi}%
       \expandafter\doprocessline
     \fi}

\fi

%D \macros
%D   {uncatcodespecials}
%D
%D This one is taken from the \TEX\ book. The \CONTEXT\
%D alternative is a bit different, but we hope this one works
%D here.

\ifx\dospecials\undefined

  \def\dospecials
    {\do\ \do\\\do\{\do\}\do\$%
     \do\#\do\^\do\_\do\&\do\%%
     \do\~\do\^^A\do\^^K} 
     
\fi 

\ifnocontextobject \uncatcodespecials \do

  \def\uncatcodespecials%
    {\def\do##1{\catcode`##1=12 }\dospecials
     \catcode`\   =\@@space
     \catcode`\^^L=\@@ignore
     \catcode`\^^M=\@@endofline
     \catcode`\^^?=\@@ignore}

\fi

\ifnocontextobject \setnaturalcatcodes \do

\def\setnaturalcatcodes%
  {\catcode`\!=\@@other \catcode`\?=\@@other \catcode`\@=\@@other
   \catcode`\#=\@@other \catcode`\&=\@@other \catcode`\|=\@@other
   \catcode`\$=\@@other \catcode`\^=\@@other \catcode`\_=\@@other
   \catcode`\*=\@@other \catcode`\/=\@@other
   \catcode`\-=\@@other \catcode`+=\@@other
   \catcode`\==\@@other \catcode`\<=\@@other \catcode`\>=\@@other
   \catcode`\"=\@@other \catcode`\'=\@@other \catcode`\`=\@@other
   \catcode`\:=\@@other \catcode`\;=\@@other
   \catcode`\,=\@@other \catcode`\.=\@@other \catcode`\~=\@@other 
   \catcode`\(=\@@other \catcode`\)=\@@other 
   \catcode`\{=\@@other \catcode`\}=\@@other
   \catcode`\\=\@@other \catcode`\%=\@@other }

\fi

%D \macros
%D   {doglobal}
%D
%D Some \CONTEXT\ low level macros can have a \type{\doglobal}
%D prefix. Let's just forget about that here:

\ifnocontextobject \doglobal \do \let\doglobal\relax  \fi

%D The next obscure one is needed in the generic verbatim
%D environment. When we end up with more of these, it's time
%D to load the module \type{syst-gen}.

\ifnocontextobject \doifincsnameelse \do

  \def\dodoifincsnameelse#1#2%
    {\def\dododoifincsnameelse##1#1##2##3\war%
       {\csname\if##2@iffalse\else iftrue\fi\endcsname}%
     \expandafter\dododoifincsnameelse#2#1@@\war}

  \long\def\doifincsnameelse#1#2#3#4%
    {\edef\@@instring{#1}%
     \expandafter\dodoifincsnameelse\expandafter{\@@instring}{#2}%
       #3%
     \else
       #4%
     \fi}

\fi

%D \macros
%D   {dostepwiserecurse, dorecurse, doloop, exitloop}
%D 
%D The next loop macro is a real weak one, and does not offer 
%D the full \CONTEXT\ functionality, let alone nesting, but 
%D for simple purposes, its behaviour is acceptable.  

\newcount\recursecounter

\def\dostepwiserecurse#1#2#3#4% very weak and rubishly version 
  {\ifnum#2<#1\relax\else\dodostepwiserecurse{#1}{#2}{#3}{#4}\fi}

\def\dodostepwiserecurse#1#2#3#4% very weak and rubishly version 
  {\recursecounter=#1\relax
   \loop 
     \edef\recurselevel{\the\recursecounter}%
     #4\relax
   \ifnum\recursecounter<#2\relax
     \advance\recursecounter by #3\relax
   \repeat}

\def\dorecurse#1%
  {\dostepwiserecurse{1}{#1}{1}}

\def\doloop%
  {\dostepwiserecurse{1}{\maxdimen}{1}}

\def\exitloop%
  {\recursecounter=\maxdimen}

%D \macros 
%D   {ifundefined,doifdefined,doifundefined,
%D    doifdefinedelse,doifundefinedelse}
%D
%D These alteratives are not robust but suitable for simple 
%D usage. The official ones are a bit faster. 

\ifnocontextobject \doifdefined \do

  \def\ifundefined#1%
    {\expandafter\ifx\csname#1\endcsname\relax}

  \def\doifdefinedelse#1#2#3%
    {\expandafter\ifx\csname#1\endcsname\relax#3\else#2\fi}

  \def\doifundefinedelse#1#2#3%
    {\expandafter\ifx\csname#1\endcsname\relax#2\else#3\fi}

  \def\doifdefined#1#2%
    {\expandafter\ifx\csname#1\endcsname\relax\else#2\fi}

  \def\doifundefined#1#2%
    {\expandafter\ifx\csname#1\endcsname\relax#2\fi}

\fi

%D \macros
%D   {doifinstringelse}
%D
%D It seems like we end up with more and more macros here. 
%D Sigh. 

\ifnocontextobject \doifinstringelse \do

  \def\p!doifinstringelse#1#2%
    {\def\pp!doifinstringelse##1#1##2##3\war%
       {\csname if\if##2@fals\else tru\fi e\endcsname}%
     \expanded{\pp!doifinstringelse#2#1@@\noexpand\war}} 

  \long\def\doifinstringelse#1#2#3#4%
    {\edef\@@@instring{#1}% 
     \@EA\p!doifinstringelse\@EA{\@@@instring}{#2}#3\else#4\fi}

\fi

%D \macros
%D   {twodigitrounding}
%D
%D We don't support rounding outside \CONTEXT. Sorry. 

\def\twodigitrounding#1{#1}

%D \macros 
%D   {lineheight}
%D
%D In \CONTEXT\ we have \type{\lineheight}, which in many 
%D cases matches \type {\baselineskip}. 

\ifnocontextobject \lineheight \do

  \def\lineheight{\baselineskip}

\fi 

%D \macros 
%D   {dohandletokens}
%D
%D The following macro is the simplified version, but good 
%D enough for day to day hacks. 
%D
%D \starttypen 
%D \dohandletokens some text\with\somemacro
%D \stoptypen 

\ifnocontextobject \dohandletokens \do

\def\dodohandletokens%
  {\ifx\next\end \else
     \docommando{\next}%
     \expandafter\dohandletokens
   \fi}

\def\dohandletokens%
  {\afterassignment\dodohandletokens\let\next= }

\long\def\handletokens#1\with#2%
  {\let\docommando=#2%
   \dohandletokens#1\end}

\fi

%D Very reduced: 

\long\def\appendtoks#1\to#2%
  {\scratchtoks{#1}\expanded{#2{\the#2\the\scratchtoks}}}

%D Well, also handy.

\def\doiffileelse#1#2#3%
  {\immediate\openin\scratchread=#1\relax
   \ifeof\scratchread
     \def\next{#3}%
   \else
     \def\next{#2}%
   \fi
   \immediate\closein\scratchread
   \next}

%D New. 

\let\donothing\empty

%D Also new: 

\def\letempty             #1{\let#1\empty}
\def\globalletempty#1{\global\let#1\empty}

\def\letvalueempty        #1{\expandafter\let\csname#1\endcsname\empty}
\def\letgvalueempty#1{\global\expandafter\let\csname#1\endcsname\empty}

%D Sigh 

\def\settrue #1{\chardef#1\zerocount}
\def\setfalse#1{\chardef#1\plusone}

\let\newconditional = \setfalse
\let\ifconditional  = \ifcase

%D That's it. Please forget this junk and take a look at how
%D it should be done.

\StopLatexHack \protect \endinput
